# Supplementary material for: Grid-Based Stochastic Model Predictive Control for Trajectory Planning in Uncertain Environments
Source: arXiv:2007.12430 source file (2021-05-14)
Supplement: Supplementary file 1 [file appendixa.tex]

% \section{Appendix A}
% \label{sec:appendixa}

% Appendixes, if needed, appear before the acknowledgment.
